# Supplementary material for: Task Specific Attention is one more thing you need for object detection
Source: arXiv:2202.09048 source file (2022-06-15)
Supplement: Supplementary file 1 [file appendix.tex]

\appendix
\section*{Appedices}
\begin{table}[hbt!]
	\caption{Comparison of TSST with state-of-the-art methods on COCO 2017 detection. }
	\centering
	\begin{tabular}{l|l|l|l}
		\toprule
		%\multicolumn{2}{c}{Part}              %     \\
		\cmidrule(r){1-2}
		Method     & Backbone     & AP$_{val}$ & AP$_{test-dev}$ \\
		\midrule
		HTC++(with instance masks)     & Swin-L & 57.1 & 57.7 \\
		DyHead     & Swin-L       & 58.4 & 58.7 \\
		TSST(ours w/o TTA)     & Swin-L       & 54.6 & 55.0 \\
		\bottomrule
	\end{tabular}
	\label{tab:table}
\end{table}
\begin{table}[hbt!]
	\caption{Complementary experiments(internal use only)}
	\centering
	\begin{tabular}{l|l|l|l}
		\toprule
		%\multicolumn{2}{c}{Part}              %     \\
		\cmidrule(r){1-2}
		Method     & Backbone     & AP$_{val}$ & AP$_{test-dev}$ \\
		\midrule

		DDETR     & r101       & 48.7 &  \\
		DDETR     & x101       & 49.0 &  \\
		DDETR     & x101-DCN       & 50.1 &  \\
		DDETR     & x101-DCN(TTA)       & 52.3 &  \\
		DDETR(ours, mmdet) & x101-DCN       & 47.6 &  \\
		DyHead     & x101-DCN       & 52.3 &  \\
		DyHead     & x101-DCN(TTA)       & 54.0 &  \\
		DyHead(ours w/o TTA)     & Swin-L       & 54.545 & \\
		TSST(ours)     & x101       & 48.7 &  \\
		TSST(ours, mmdet)     & x101-DCN       & 49.0 &  \\
		TSST(ours w/o TTA)     & Swin-L       & 54.6 & 55.0 \\
		\bottomrule
	\end{tabular}
	\label{tab:table}
\end{table}
